# Supplementary material for: Maya: Falsifying Power Sidechannels with Dynamic Control
Source: arXiv:1907.09440 source file (2019-08-18)
Supplement: Supplementary file 1 [file appendix.tex]

\section{Robust Controller Design}
\label{app_robust}
